# Supplementary material for: A Survey on Test-Time Scaling in Large Language Models: What, How, Where, and How Well?
Source: arXiv:2503.24235 source file (2025-05-04)
Supplement: Supplementary file 1 [file tune.tex]

\section{Details on Tuning-based Approaches}
\label{app:tuning}

\subsection{Supervised Finetuning (SFT)}
\label{app:sft}
Training an LLM via next-token prediction on synthetic or distilled long CoTs enables it to internalize structured reasoning patterns and effectively “think” through complex problems. By mimicking extended rationales, SFT reduces the reliance on explicit prompting at inference time. 

\subsection{Reinforcement Learning (RL)}
\label{app:rl}

\subsubsection{Reward Model-free Methods}
Recent advancements in RL and preference optimization have significantly enhanced LLM performance in reasoning tasks. 
A key development is RL with verifiable reward, introduced by DeepSeek R1~\citep{deepseek-r1}, which uses rule-based reward mechanisms to ensure dense feedback. 
Subsequent methods like cDPO~\citep{lin2024critical}, CPL~\citep{wang2024cpl}, Focused-DPO~\citep{zhang2025focused}, DAPO~\citep{liu2024improvingmultistepreasoningabilities}, and RFTT~\citep{zhang2025reasoning} emphasize preference optimization for critical or error-prone regions, enhancing internal scaling and improving accuracy. 
Selective DPO~\citep{gao2025principled} matches data difficulty to model capacity. 
SimPO~\citep{meng2024simpo} removes the reference model in DPO, using the average log probability of a sequence as an implicit reward.

In mathematical problem-solving, DQO~\citep{ji2024enhancing} and OREO~\citep{wang2024offline} use novel value function techniques. Open-source training frameworks, such as SimpleRL~\citep{zeng2025simplerl} and DeepScaler~\citep{deepscaler2025}, replicate the technology stack of DeepSeek R1. Others, like X-R1~\citep{xr12025} and TinyZero~\citep{tinyzero}, prioritize cost-effectiveness. Open-Reasoner-Zero~\citep{OpenReasonerZero2025} uses a 32B model to replicate DeepSeek R1-zero. Finally, frameworks like OpenR~\citep{wang2024openr}, OpenRLHF~\citep{hu2024openrlhf}, OpenR1~\citep{openr1}, and Logic-RL~\citep{xie2025logic} have further simplified replication of internal-scaling RL methods.

\subsubsection{Reward Model-based Methods}
Relying on a learned reward model, typically a Bradley-Terry formulation~\citep{zheng2023secrets} guided by human preferences, Proximal Policy Optimization (PPO)~\citep{schulman2017proximalpolicyoptimizationalgorithms} is widely used. 
Follow-up work includes ReMax~\citep{li2023remax}, which introduces variance-reduction techniques, and GRPO~\citep{shao2024deepseekmath}, which streamlines value models for faster training. 
REINFORCE++~\citep{hu2025reinforce++}, DVPO~\citep{huang2025lean}, PRIME~\citep{cui2025process}, and SPPD~\citep{yi2025sppd} all improve upon or simplify these actor-critic frameworks. 
Recent efforts address the challenges of reward model quality and training stability: UGDA~\citep{sun2025uncertain} refines the reward model, VinePPO~\citep{kazemnejad2024vineppo} uses unbiased Monte Carlo estimates, LCPO~\citep{aggarwal2025l1} balances accuracy with length constraints, and Rest-MCTS*~\citep{zhang2024rest} adopts tree-search-based RL for step-wise training signals.

Collectively, these refinements and frameworks highlight the potential of RL-based approaches to yield more robust, accurate, and computationally efficient internal scaling for LLMs.
